# Supplementary material for: Mixed-integer linear representability, disjunctions, and Chvatal functions --- modeling implications
Source: arXiv:1711.07028 source file (2017-11-19)
Supplement: Supplementary file 1 [file appendix.tex]

% !TEX root = ../journal-submission.tex

\section{The variable elimination method of Williams and Hooker \cite{williams-hooker}}\label{app:w-h-variable-elimination-method}

\chris{Mention somewhere that we don't use the Chinese remainder in our results to simplify things.}

The appendix gives a formal description of the method of Williams and Hooker in \cite{williams-hooker}. We begin with the process of eliminating a single variable. Consider a set of the following form
\begin{align*}
F = \{x = (x_1, \ldots, x_n) \in \mathbb{Z}^n: ~ a^i x \leq b^i, i \in I, ~ c^j x \equiv d^j \mod m^j, j \in J \}
\end{align*}
where $a^i \in \mathbb{Z}^n, b^i \in \mathbb{Z}, \;\;\forall i \in I$, and $c^j \in \mathbb{Z}^n, d^j \in \mathbb{Z}, m^j \in \mathbb{Z},\;\; \forall j \in J.$ 
We adapt the Fourier-Motzkin elimination method to describe the projection of $F$ onto $x_{-1} = (x_2, \ldots, x_n)$. 

\subsection{Transform into standard form}
Define the following sets according the coefficients on the variable $x_1$: $P = \{p \in I : ~  a_1^p > 0 \}$,
$N = \{ n \in I : ~ a_1^n < 0\}$, $R = \{j \in J : ~ c_1^j \neq 0 \}$. We use these sets to classify the
constraints of $F$ as:
\begin{align}
a^p x & \leq b^p,  \phantom{ \bmod m^j } \text{ \ \ \ } \forall p \in P   \tag{L}  \label{eq:positive-coefficients} \\
a^n x & \leq b^n,  \phantom{ \bmod m^j } \text{ \ \ \ } \forall n \in N   \tag{G}  \label{eq:negative-coefficients} \\
c^j x & \equiv d^j \bmod m^j,  \text{ \ \ } \forall j \in R \tag{M} \label{eq:congruences}
\end{align}
and the remaining constraints of $F$ are collected as:
\begin{align}\label{eq:left-overs}
\begin{split}
a^i_{-1} x_{-1} & \leq b^i,   \phantom{ \bmod m^j }  \text{\ \ \ \ } \forall i \in I \setminus (P \cup N) \\
c_j^{-1} x_{-1} & \equiv d^j \bmod m^j,  \text{\ \ } \forall j \in J \setminus R.
\end{split}
\tag{Z}
\end{align}
%
% Define the set of constraints $L, G, M, Z$ from the constraints in $F$ as the following:
% \begin{align*}
%   L : ~ &  a^p x \leq b^p, \;\; p \in P, a_1^p > 0, \text{ where } P \subseteq I, \\
%   G : ~ &  a^n x \leq b^n, \;\; n \in N, a_1^n < 0, \text{ where } N \subseteq I, \\
%   M : ~ &  c^j x \equiv d^j \mod m^j, \;\; j \in R, \text{ where } c_1^j \neq 0, R \subseteq J \\
%   Z : ~ &  \text{the rest of constraints where } x_1 \text{ has 0 coefficient},
% \end{align*}
Therefore, we can rewrite $F$ as: \begin{align*}
  F  = & \left\{ x \in \mathbb{Z}^n : ~
  \begin{array}{lll}
  a_1^p x_1 + a_{-1}^p x_{-1} &\leq b^q, &  \forall p \in P \\
  a_1^n x_1 + a_{-1}^n x_{-1} &\leq b^n, &  \forall n \in N \\
  c^j_1 x_1 + c^j_{-1} x_{-1} &\equiv d^j  \mod m^j, & \forall j \in R \\
   & \eqref{eq:left-overs} & \\
  \end{array}
  \right\}.\\
  = & \{x \in \mathbb{Z}^n : ~ \eqref{eq:positive-coefficients}, \eqref{eq:negative-coefficients}, \eqref{eq:congruences} ,\eqref{eq:left-overs}\}
\end{align*}

\subsection{Project onto $x_{-1}$ by Fourier elimination method}
In order to project $F$ onto $x_{-1}$ by Fourier elimination method, we need to consider the following three cases that consider different scenarios of when the index sets $P$, $N$, and $R$ are empty or nonempty.
\subsubsection{Case 1: $P \neq \emptyset$ and $N\neq \emptyset$}
\textbf{Show with less slack variables and written with notation in the form of vectors.}\\
\textbf{Some Notations:}\\
Let $q = \text{l.c.m}( \{a_1^p \}_{p \in P}, \{-a_1^n\}_{n \in N}, \{|c_1^j|\}_{j \in R})$ \guanyi{just to be the same with $\{|c_1^j|\}_{j \in R}$ in case 2, and this change will ensure $q$ be positive} and define
\begin{align*}
\begin{array}{lll}
  \bar{a}_{-1}^p &= \frac{q}{a_1^p} a_{-1}^p, & \forall p \in P, \\
  \bar{b}^p& = \frac{1}{a_1^p} b^p, & \forall p \in P, \\
  \bar{a}_{-1}^n &= \frac{q}{-a_1^n} a_{-1}^n, & \forall n \in N, \\
  \bar{b}^n& = \frac{1}{-a_1^n} b^n, & \forall n \in N, \\
  \bar{c}_{-1}^j&  = \frac{q}{c_1^j} c_{-1}^j, & \forall j \in R, \\
  \bar{d}^j & = \frac{q}{c_1^j}d^j, & \forall j \in R, \\
  \bar{m}^j & =  \frac{q}{c_1^j} m^j, & \forall j \in R, \\
  m & = \text{l.c.m}(q, \{\bar{m}^j\}_{j \in R}), &
\end{array}
\end{align*}
Define slack variables $s^1_p, s^1$ that we use to eliminate the first variable $x_1$ as:
\begin{align*}
\begin{array}{lll}
  s^1_p & \in \mathbb{Z}_+, \forall p \in P, & \text{ slack variables ,} \\
  s^1 & = (s^1_p)_{p \in P} \in \mathbb{Z}_+^{|P|}, & \text{ vector of slack variables.}
\end{array}
\end{align*}

\begin{theorem} Suppose $P \neq \emptyset$ and $N\neq \emptyset$.
Then the projection of $F$ onto $x_{-1}$ is
\begin{align*}
  & \Proj_{x_{-1}} (F) = \\
  &  \bigcup_{s^1 \in \mathbb \{0, 1, \ldots, m-1\}^{|N|}}
  \left\{ x_{-1} \in \mathbb{Z}^{n-1}: ~
  \begin{array}{lll}
  \bar{a}_{-1}^p x_{-1} + \bar{a}_{-1}^n x_{-1} \leq \bar{b}^p + \bar{b}^n - s^1_p & & \forall p \in P, \forall n \in N \\
  \bar{c}_{-1}^j x_{-1} - \bar{a}_{-1}^p x_{-1} \equiv \bar{d}^j - \bar{b}^p + s^1_p & \mod \bar{m}^j, & \forall j \in R, \forall p \in P \\
  -\bar{a}_{-1}^p x_{-1} \equiv - \bar{b}^p + s^1_p & \mod q, & \forall p \in P \\
   \eqref{eq:left-overs} & & \\
  \end{array}
  \right\}.
\end{align*}
\kipp{do we use the index $r$ or $u_{1,p,n}$} \amitabh{I think we definitely want $u_{1,p,n}$ because we don't want all slack variables to have the same value, and this interpretation is possible if the same letter $r$ is used for all of them.} \chris{What does the notation mean to be $\forall n \in N$ on top of unions? I have never seen that notation before.}
\end{theorem}
\begin{proof}
\textbf{First: Show that the projection $\text{Proj}_{x_{-1}}(F)$ can be written as the union of infinitely many disjunctions.}\\
Rewrite set $F$ as
\begin{align*}
  F = & \left\{ x \in \mathbb{Z}^n : ~
  \begin{array}{lll}
  qx_1 \leq \bar{b}^p - \bar{a}_{-1}^p x_{-1}, & & \forall p \in P \\
  -\bar{b}^n + \bar{a}_{-1}^n x_{-1} \leq q x_1, & & \forall n \in N \\
  qx_1 \equiv \bar{d}^j - \bar{c}_{-1}^j x_{-1} & \mod \bar{m}^j, & \forall j \in R \\
   \eqref{eq:left-overs} & & \\
  \end{array}
  \right\} \\
  = & \left\{ x \in \mathbb{Z}^n : ~
  \begin{array}{lll}
  -\bar{b}^n + \bar{a}_{-1}^n x_{-1} \leq qx_1 \leq \bar{b}^p - \bar{a}_{-1}^p x_{-1}, & &\forall p \in P, \forall n \in N \\
  qx_1 \equiv \bar{d}^j - \bar{c}_{-1}^j x_{-1} & \mod \bar{m}^j, & \forall j \in R \\
   \eqref{eq:left-overs} & & \\
  \end{array}
  \right\}
\end{align*}
By adding auxiliary variables \kipp{do want $u_1$ or $u_{1,p,n}$}\amitabh{I think we want $u_{1,p,n}$ -- see my comment above}  $s^1_p \in \mathbb{Z}_{+}, ~ \forall p \in P$ as we defined above, and let $qx_1 = \bar{b}^p - \bar{a}_{-1}^p x_{-1} - s^1_p$. \guanyi{we could also add auxiliary variables $u_{1,p}$, I think in order to improve the efficiency, maybe we need to compare the cardinalities of set $P$ and $N$ before each step} Therefore the projection of $F$ onto $x_{-1}$ is
\begin{align*}
  & \Proj_{x_{-1}} (F) = % \bigcup_{u_{1,n,p} \in \mathbb{Z}_{+}}^{ \forall n \in N, \forall p \in P}
 \bigcup_{s^1 \in \mathbb Z_{+}^{|P|}} F'( s^1 )
\end{align*}
where $s^1 = (s^1_p)_{p \in P}$ is defined as above and
\begin{align}
 F'(s^1) & =  \left\{ x_{-1} \in \mathbb{Z}^{n-1}: ~
  \begin{array}{lll}
  \bar{a}_{-1}^p x_{-1} + \bar{a}_{-1}^n x_{-1} \leq \bar{b}^p + \bar{b}^n - s^1_p & & \forall p \in P, \forall n \in N \\
  \bar{c}_{-1}^j x_{-1} - \bar{a}_{-1}^p x_{-1} \equiv \bar{d}^j - \bar{b}^p + s^1_p & \mod \bar{m}^j, & \forall j \in R, \forall p \in P \\
  -\bar{a}_{-1}^p x_{-1} \equiv - \bar{b}^p + s^1_p & \mod q, & \forall p \in P \\
   \eqref{eq:left-overs} & & \\
  \end{array}
  \right\}
\end{align}
\guanyi{We should write the following property as a theorem: see Theorem 1.3 below}\\
\textbf{Note:} Since both the coefficients of variables and the coefficients of modulus are independent from slack variables $s^1_p, \forall p \in P$, then the different choices of values of slack variables only influence the values of constants in each disjunctions $F'(s^1)$. Therefore, if we do Fourier-Motzkin elimination method for the second variable $x_2$ on $\text{Proj}_{x_{-1}}(F)$, we have the least common multiplier $q$ for each disjunctions remain the same, since for each disjunction, the coefficients of $x_2$ are same i.e., independent from the slack variables $s^1_p, \forall p \in P$. Therefore, for each disjunctions, the value of $m$ as we defined above, remain the same. Then we have the property that, in the step of eliminate $x_2$, although we need to add slack variables for each disjunctions for $\text{Proj}_{x_{-1}} (F)$, the range of these slack variables are the same since $m$ remain the same.\\
\textbf{Second: Show that the projection $\text{Proj}_{x_{-1}}$ can be simplified as the union of finitely many disjunctions.}\\
Let $m = \text{l.c.m}(q, \{\bar{m}^j\}_{j \in R})$ as we defined above. Let $\bmod(z,  m)$ denotes the integer that $z$ is reduced modulo $m$ to a unique integer in $\{0, 1, \ldots,  m - 1 \}.$ For an arbitrary, but fixed $\hat{s}^1_p \in \Z_{+}$, $$\begin{array}{rl} & \{x_{-1} \in \mathbb{Z}^{n-1}: -\bar{b}^n + \bar{a}_{-1}^n x_{-1} \leq \bar{b}^p - \bar{a}_{-1}^p x_{-1} - \hat{s}^1_p,\;\; \forall p \in P, \forall n \in N \} \\
= & \{x_{-1} \in \mathbb{Z}^{n-1}: \bar{a}_{-1}^p x_{-1} + \bar{a}_{-1}^n x_{-1} \leq \bar{b}^p + \bar{b}^n - \hat{s}^1_p,\;\; \forall p \in P, \forall n \in N \} \\
\subseteq & \{x_{-1} \in \mathbb{Z}^{n-1}: -\bar{b}^n + \bar{a}_{-1}^n x_{-1} + \leq \bar{b}^p - \bar{a}_{-1}^p x_{-1} - (\hat{s}^1_p \mod m),\;\; \forall p \in P, \forall n \in N \} \\
= & \{x_{-1} \in \mathbb{Z}^{n-1}: \bar{a}_{-1}^p x_{-1} + \bar{a}_{-1}^n x_{-1} \leq \bar{b}^p + \bar{b}^n - (\hat{s}^1_p \mod m),\;\; \forall p \in P, \forall n \in N \}.
\end{array}$$
Combining this observation with Lemma~\ref{lemma:cong-reduction-2} in the appendix, we obtain that $F'(\hat{s}^1) \subseteq F'(\bmod(\hat{s}^1,m))$ for any $\hat{s}^1 \in \Z_{+}^{|P|}$. Therefore,

%Using  Lemma~\ref{lemma:cong-reduction-2} as in Cases 1 and 2 gives
\begin{eqnarray*}
  \Proj_{x_{-1}} (F) =  \bigcup_{s^1 \in \mathbb Z_{+}^{|P|}} F'( \hat{s}^1 ) \subseteq  \bigcup_{s^1 \in \mathbb \{0, 1, \ldots, m-1\}^{|P|}} F'( s^1 ).
\end{eqnarray*}
\end{proof}
%For any $u_{1,p,n} \in \mathbb{Z}$, we have
%\begin{align*}
%  & \left\{ x_{-1} \in \mathbb{Z}^{n-1}: ~
%  \begin{array}{lll}
%  -\bar{b}^n + \bar{a}_{-1}^n x_{-1} + ( u_{1,p,n} + m ) \leq \bar{b}^p - \bar{a}_{-1}^p x_{-1}, & & \forall p \in P, n \in N \\
%  -\bar{b}^n + \bar{a}_{-1}^n x_{-1} + ( u_{1,p,n} + m )\equiv \bar{d}^j - \bar{c}_{-1}^j x_{-1} & \mod \bar{m}^j, & \forall j \in R, p \in P, n \in N \\
%  -\bar{b}^n + \bar{a}_{-1}^n x_{-1} + ( u_{1,p,n} + m )\equiv 0 & \mod q, & \forall p \in P, n \in N \\
%  Z & & \\
%  \end{array}
%  \right\} \\
%  \subseteq & \left\{ x_{-1} \in \mathbb{Z}^{n-1}: ~
%  \begin{array}{lll}
%  -\bar{b}^n + \bar{a}_{-1}^n x_{-1} + u_{1,p,n} \leq \bar{b}^p - \bar{a}_{-1}^p x_{-1}, & & \forall p \in P, n \in N \\
%  -\bar{b}^n + \bar{a}_{-1}^n x_{-1} + u_{1,p,n} \equiv \bar{d}^j - \bar{c}_{-1}^j x_{-1} & \mod \bar{m}^j, & \forall j \in R, p \in P, n \in N \\
%  -\bar{b}^n + \bar{a}_{-1}^n x_{-1} + u_{1,p,n} \equiv 0 & \mod q, & \forall p \in P, n \in N \\
%  Z & & \\
%  \end{array}
%  \right\},
%\end{align*}

\subsubsection{Case 2: $P = \emptyset$ or $N = \emptyset$, and $R \neq \emptyset$.}
\begin{theorem}
Let $P = \emptyset$ or $N = \emptyset$, and $R \neq \emptyset$. Let  $q = \text{l.c.m} \{\,|c_1^j|,\;\; j \in R\}$, let $r \in R$ be the index in $R$ that we will use in further proof  \chris{Why use absolute values here and not in the statment of the previous theorem?} and define
\begin{align*}
\begin{array}{lll}
  \bar{d}^j & = \frac{q}{c_1^j} d^j,  & \forall j \in R,\\
  \bar{c}_{-1}^j & = \frac{q}{c_1^j} c_{-1}^j,  & \forall j \in R,\\
  \bar{m}^j & = \frac{q}{c_1^j} m^j,  & \forall j \in R, \\
  m & = \text{l.c.m}(q, \{\bar{m}^j\}_{j \in (R \backslash \{r\})}), & \\
\end{array}
\end{align*}
Define slack variables $s^1 \in \mathbb{Z}$ that we used to eliminate the first variable $x_1$.

Let $r\in R$ be any element. The projection of $F$ onto $x_{-1}$ is
\begin{align*}
  & \Proj_{x_{-1}} (F) \\
  = & \bigcup_{s^1 \in \{ 0, \ldots , m - 1 \} }\left\{ x_{-1} \in \mathbb{Z}^{n-1}: ~
  \begin{array}{ll}
  \bar{c}_{-1}^j x_{-1} - \bar{c}_{-1}^r x_{-1} \equiv \bar{d}^j - \bar{d}^r - s^1 \bar{m}^r & \mod \bar{m}^j, \;\; \forall j \in R\setminus\{r\} \\
   - \bar{c}_{-1}^r x_{-1} \equiv - \bar{d}^r - s^1 \bar{m}^r & \mod q \\
   \eqref{eq:left-overs} & \\
  \end{array}
  \right\}.
\end{align*}
\kipp{should we use a subscript $r$ or $u_{1}$ in the union above?} \chris{I like $u_1$ for bookkeeping purposes. I think when we iterate to project our more than one variable we will want these subscripts to help us keep track of what is happening.}
\end{theorem}

\begin{proof}
\textbf{First: Show that the projection $\text{Proj}_{x_{-1}}(F)$ can be written as the union of infinitely many disjuncions.}\\
Consider the congruence corresponding to $r\in R$, $\{x \in \Z^n: c^r_1x_1 + c^r_{-1}x_{-1} \equiv d^r \mod m^r\}$. We scale this congruence, and add a slack variable $s^1\in \Z$ to express the congruence as \begin{equation}\label{eq:re-express}\{x \in \Z^n: c^r_1x_1 + c^r_{-1}x_{-1} \equiv d^r \mod m^r \}= \cup_{s^1\in \Z}\{ x \in \Z^n: qx_1 = \bar{d}^r - \bar{c}_{-1}^r x_{-1} + s^1 \bar{m}^r \}.\end{equation}
If we set $F' := \{x \in \Z^n: \eqref{eq:congruences}, \eqref{eq:left-overs}\}$, then by substituting out $x_1$ using~\eqref{eq:re-express}, we obtain that \begin{equation}\label{eq:infinite-union}\Proj_{x_{-1}} (F') = \bigcup_{s^1 \in \mathbb{Z}} F'(s^1),\end{equation} where \begin{align*}
F'(u_1) :=  & \left\{ x_{-1} \in \mathbb{Z}^{n-1}: ~
  \begin{array}{ll}
  \bar{c}_{-1}^j x_{-1} - \bar{c}_{-1}^r x_{-1} \equiv \bar{d}^j - \bar{d}^r - s^1 \bar{m}^r & \mod \bar{m}^j, \;\; \forall j \in R\setminus\{r\} \\
   - \bar{c}_{-1}^r x_{-1} \equiv - \bar{d}^r - s^1 \bar{m}^r & \mod q \\
   \eqref{eq:left-overs} & \\
  \end{array}
  \right\}
\end{align*}
We now claim that
\begin{align*}
\Proj_{x_{-1}}(F) = \Proj_{x_{-1}} (F').
\end{align*}
Since we have dropped constraints going from $F$ to $F'$, $\Proj_{x_{-1}}(F) \subseteq \Proj_{x_{-1}} (F')$ is trivially true. If $P \cup N = \emptyset$, then the reverse inclusion is also trivial. If $P \neq \emptyset$, then for any $\hat x_{-1}$ in the right hand side, one can find a small enough $\hat x_1$ such that $(\hat x_1, \hat x_{-1})$ satisfies all the constraints indexed by $P$. Similarly, for the case $N \neq \emptyset$.\\
\guanyi{We should write the following property as a theorem: See Theorem 1.3 below}\\
\textbf{Note: } Similarly, since both the coefficients of variables and the coefficients of modulus are independent from slack variables $s^1$ like Case 1, the different choices of slack variables only influence the values of constants on the right hand side of constraints. Therefore, if we do Fourier-Motzkin elimination method for the second variable $x_2$ on $\text{Proj}_{x_{-1}}(F)$, we have the least common multiplier $q$ for each disjunctions remain the same, since for each disjunction, the coefficients of $x_2$ are same, i.e., independent from the slack variable $s^1$. Therefore, for each disjunctions, the value of $m$ as we defined above, remain the same. Then we have the property that, in the step of eliminate $x_2$, although we need to add slack variables for each disjunctions for $\text{Proj}_{x_{-1}} (F)$, the range of these slack variables are the same since $m$ remain the same.\\
\textbf{Second: show that the infinite union in~\eqref{eq:infinite-union} can be expressed by a finite union.}\\
Let $m = \text{l.c.m}(q, \{\bar{m}^j\}_{j \in (R \backslash \{r\}) })$ as we defined above.  For an arbitrary, but fixed $\hat{s}^1 \in \mathbb{Z},$ Lemma~\ref{lemma:cong-reduction-2} implies that $F'(\hat{s}^1)  = F'(\hat{s}^1 \bmod m)$.  Since  $(\hat{s}^1 \bmod m) \in \{0, 1, \ldots,   m -1\}$  we have \chris{We have introduced conflicting notation for $\hat{u}_1 \bmod m$ and $\bmod(\hat u_1, m)$ (see in the notation leading up to Lemma~2.1). Which do we prefer, which is more standard? I always thought the unary use of mod like 8 mod 2 always gives a number between $0$ and $1$. Any thoughts?}
\begin{eqnarray*}
F'(\hat{s}^1) \subseteq  \bigcup_{s^1 \in \{0,\ldots, m-1\}} F'( s^1 ).
\end{eqnarray*}
\kipp{should we use a subscript $r$ or $u_{1}$ in the union above?} But $\hat s^{1}$ was an arbitrary element of $\mathbb Z$ so this containment is valid for all $s^{1} \in \mathbb Z$ which implies
\begin{eqnarray*}
  \Proj_{x_{-1}} (F) =  \Proj_{x_{-1}} (F') = \bigcup_{s^{1} \in \mathbb Z}F'( s^{1} ) =  \bigcup_{s^1 \in \{ 0, \ldots,  m - 1 \} } F'( s^1 ).
\end{eqnarray*}
We have arrived at the conclusion of the theorem.\end{proof}

\subsubsection{Case 3: $P\cup N \cup R = \emptyset$.} In this case, $x_1$ has 0 coefficient in all constraints. Therefore,
\begin{align*}
\Proj_{x_{-1}}(F) = \{x_{-1} \in \Z^{n-1}:  \eqref{eq:left-overs}\}.
\end{align*}

\subsubsection{Insight}
\begin{theorem}
The range of slack variables in each iteration of Fourier-Motzkin elimination method is the same across disjunctions in Case 1 and Case 2.
\end{theorem}
\begin{proof}
\textbf{Case 1:}\\
By Theorem 1.1, we have:
\begin{align*}
  & \Proj_{x_{-1}} (F) = \\
  &  \bigcup_{s^1 \in \mathbb \{0, 1, \ldots, m-1\}^{|N|}}
  \left\{ x_{-1} \in \mathbb{Z}^{n-1}: ~
  \begin{array}{lll}
  \bar{a}_{-1}^p x_{-1} + \bar{a}_{-1}^n x_{-1} \leq \bar{b}^p + \bar{b}^n - s^1_p & & \forall p \in P, \forall n \in N \\
  \bar{c}_{-1}^j x_{-1} - \bar{a}_{-1}^p x_{-1} \equiv \bar{d}^j - \bar{b}^p + s^1_p & \mod \bar{m}^j, & \forall j \in R, \forall p \in P \\
  -\bar{a}_{-1}^p x_{-1} \equiv - \bar{b}^p + s^1_p & \mod q, & \forall p \in P \\
   \eqref{eq:left-overs} & & \\
  \end{array}
  \right\}.
\end{align*}
Consider one disjunction $F'(s^1)$ in this projection, define:
\begin{align*}
\begin{array}{llll}
  A_{-1}^{\ast} & = (\bar{a}^p_{-1} + \bar{a}^n_{-1})_{\forall p \in P, \forall n \in N} & \in \mathbb{Z}^{(n-1) \times (|P||N|)}, &\text{ coefficients of inequalities}\\
  C_{-1}^{\ast} & = 
  \left(
  \begin{array}{cc}
  \bar{c}_{-1}^j - \bar{a}_{-1}^p \\
  -\bar{a}_{-1}^p \\
  \end{array}
  \right) & \in 
  \left(
  \begin{array}{cc}
  \mathbb{Z}^{(n-1) \times (|R||P|)} \\
  \mathbb{Z}^{(n-1) \times (|P|)} \\
  \end{array}
  \right), & \text{ coefficients of congruences} \\
  m_{-1}^{\ast} & = 
  \left(
  \begin{array}{cc}
  \bar{m}^j \\
  q \\
  \end{array}
  \right) & \in
  \left( 
  \begin{array}{cc}
  \mathbb{Z}^{1 \times (|R||P|)} \\
  \mathbb{Z}^{1 \times (|P|)} \\
  \end{array}
  \right),& \text{ coefficients of modulus}\\
  b_{-1}^{\ast} (s^1) & = (\bar{b}^p + \bar{b}^n - s^1_p)_{\forall p \in P, \forall n \in N} & \in \mathbb{Z}^{(|P||N|) \times 1}, & \text{ constants of inequalities}\\
  d_{-1}^{\ast} (s^1) & = 
  \left(
  \begin{array}{cc}
  \bar{d}^j - \bar{b}^p + s^1_p \\
  - \bar{b}^p + s^1_p \\
  \end{array}
  \right) & \in 
  \left(
  \begin{array}{cc}
  \mathbb{Z}^{(|R||P|) \times 1} \\
  \mathbb{Z}^{|P|} \\
  \end{array}
  \right), & \text{ constants of congruences}
\end{array}
\end{align*}
where $A_{-1}^{\ast}, C_{-1}^{\ast}, m_{-1}^{\ast}$ are independent from the slack variable $s^1$, i.e., the same among each disjunction $F'(s^1)$ and $b_1(s^1)^{\ast}, d_{-1} (s^1)^{\ast}$ are linear functions about $s^1$. Note that the definition of $\eqref{eq:left-overs}$ is the set of constraints with 0 coefficient of $x_1$ in original set $F$. Since $\eqref{eq:left-overs}$ is the set independent from slack variables $s^1$, then combine the coefficients of constraints in $\eqref{eq:left-overs}$ with $A_{-1}^{\ast}, C_{-1}^{\ast}, m_{-1}^{\ast}, b_1(s^1)^{\ast}, d_{-1} (s^1)^{\ast}$ and denote the combined set as $A_{-1}, C_{-1}, m_{-1}, b_1(s^1), d_{-1} (s^1)$. Therefore, we can write $F'(s^1)$ as:
\begin{align*}
  F'(s^1) = 
  \left\{ x_{-1} \in \mathbb{Z}^{n - 1}:~ 
  \begin{array}{lll}
  A_{-1} x_{-1} \leq b_{-1}(s^1)& \\
  C_{-1} x_{-1} \equiv d_{-1}(s^1)& \bmod ~ m_{-1} \\
  \end{array}
  \right\}.
\end{align*}
And define sets according the coefficients on the variables $x_2: ~ P_{2}, N_{2}, R_{2}$ as we did for set $P,N,R$. And the remaining constraints of $F'(s^1)$ are collected in set $\eqref{eq:left-overs}$, where this $\eqref{eq:left-overs}$ denotes the set of constraints with 0 coefficient for variable $x_2$. Transform $F'(s^1)$ into standard form based on the coefficient of $x_2$ as:
\begin{align*}
  F'(s^1)  = & \left\{ x_{-1} \in \mathbb{Z}^{n-1} : ~
  \begin{array}{lll}
  a_2^p x_2 + a_{-2}^p x_{-2} &\leq b_{-1}^q(s^1), &  \forall p \in P_{2} \\
  a_2^n x_2 + a_{-2}^n x_{-2} &\leq b_{-1}^n(s^1), &  \forall n \in N_{2} \\
  c^j_2 x_2 + c^j_{-2} x_{-2} &\equiv d_{-1}^j(s^1)  \mod m_{-1}^j, & \forall j \in R_{2} \\
   & \eqref{eq:left-overs} & \\
  \end{array}
  \right\}.
\end{align*}
Note that the coefficient $\{a_2^p\}_{\forall p \in P_{2}}, ~ \{a_2^n\}_{ \forall n \in N_{2}}, ~ \{c_2^j\}_{\forall j \in R_2}, \{m_{-1}^j\}_{j \in R_2}$ are independent from the slack variables $s^1$. Then the standard sets $P_2, N_2, R_2$ are independent from  slack variables $s^1$. Then for each disjunctions $F'(s^1)$, the least common multiplier $q_2$ are the same since $q_2 = \text{l.c.m}( \{a_2^p \}_{p \in P_2}, \{-a_2^n\}_{n \in N_2}, \{|c_2^j|\}_{j \in R_2})$ which also independent from $s^1$. Therefore, the set of modulus $\{\bar{m}^j_{-1}\}_{j \in R_2} = \{ \frac{q_2}{c_2^j} m_{-1}^j \}_{j \in R_2}$ after scalaring is independent from $s^1$. Therefore, we have the range $m_2$ of slack variable $s^2$ is independent from $s^1$ since $m_2 = \text{l.c.m} ( q_2, \{\bar{m}_{-1}^j\}_{j \in R_2} )$ is independent from $s^1$.\\

\textbf{Case 2:} Similarly.
\end{proof}

\subsection{Conclusion}
Combine three cases above, we can project the original set $F$ onto $\Proj_{x_{-1}}(F)$ using Fourier-Motzkin type of elimination.

\subsection{Projecting out several variables}
Still consider a set of the following form
\begin{align*}
F = \{x = (x_1, \ldots, x_n) \in \mathbb{Z}^n: ~ a^i x \leq b^i, i \in I, ~ c^j x \equiv d^j \mod m^j, j \in J \}
\end{align*}
where $a^i \in \mathbb{Z}^n, b^i \in \mathbb{Z}, \;\;\forall i \in I$, and $c^j \in \mathbb{Z}^n, d^j \in \mathbb{Z}, m^j \in \mathbb{Z},\;\; \forall j \in J.$ We adapt the Fourier-Motzkin elimination method to describe the projection of $F$ onto $x_{-k} = (x_{k+1}, \ldots, x_n)$, i.e, we project out $x_1, x_2, \ldots, x_k$.\\
\textbf{Notations:}\\
Let $i$th iteration of Fourier-Motzkin elimination method denotes the projection of $\text{Proj}_{x_{-(i-1)}}(F)$ onto $x_{-i}$ and get $\text{Proj}_{x_{-i}} (F)$, i.e., project out $x_i$. \\
Let $q_i, \forall i = 1, \ldots, k$ be the least common multiplier $q$ as we define in Case 1 and Case 2 of the $i$th iteration of Fourier-Motzkin elimination method to project out variable $x_i$. \guanyi{By Note, we should write this as a theorem}By Theorem 1.3,  let $m_i, \forall i =1, \ldots, k$ be the least common multiplier $m$ as we define in Case 1 and Case 2 of the $i$th iteration of Fourier-Motzkin elimination method. Let $s^1, \ldots s^k$ be a sequence of vectors of slack variables where $s^i, \forall i =1,\ldots,k$ be the vector of slack variables of $i$th iteration of Fourier-Motzkin elimination method. Let $A_{-k}, C_{-k}$ be the set of coefficients of variable $x_{-k}$ in inequality constraints and congruences constraints and $\bar{m}_{-k}$ be the set of coefficients of modulus in congruences constraints. Let $b_{-k}(s^1, \ldots, s^k), d_{-k}(s^1, \ldots, s^k)$ be two sets of linear functions for the vectors $s^1, \ldots, s^k$ of slack variables.
\begin{theorem}
The projection of $F$ onto $x_{-k}$ is
\begin{align*}
  & \text{Proj}_{x_{-k}} (F)\\
  = & \bigcup_{s^i \in \{0, 1, \ldots, m_i - 1\}^{|P_i|}}^{i \in \{1,\ldots, k\}}
  \left\{ x_{-k} : ~
  \begin{array}{ll}
  A_{-k} x_{-k} \leq b_{-k}(s^1, \ldots, s^k) & \\
  C_{-k} x_{-k} \equiv d_{-k}(s^1, \ldots, s^k)& \bmod \bar{m}_{-k}
  \end{array}
  \right\}
\end{align*}
where $A_{-k}, C_{-k}, \bar{m}_{-k}$ do not depend on $s^1, \ldots, s^k$ and $b_{-k}(s^1, \ldots, s^k),  d_{-k}(s^1, \ldots, s^k)$ are linear functions for $s^1, \ldots, s^k$.
\end{theorem}
\begin{proof}
By Theorem 1.1, the Projection of $F$ onto $x_{-1}$ is 
\begin{align*}
  \text{Proj}_{x_{-1}} (F) = \bigcup_{s^1 \in \{0, 1, \ldots, m_1 - 1\}^{|P_1|}} F'(s^1).
\end{align*}
Then by the proof of Theorem 1.3, we have 
\begin{align*}
  F'(s^1) =
  \left\{ x_{-1} \in \mathbb{Z}^{n - 1}:~
  \begin{array}{lll}
  A_{-1} x_{-1} \leq b_{-1}(s^1)& \\
  C_{-1} x_{-1} \equiv d_{-1}(s^1)& \bmod ~ m_{-1} \\
  \end{array}
  \right\}
\end{align*}
where $A_{-1}, C_{-1}, m_{-1}, b_{-1}(s^1), d_{-1}(s^1)$ are the same as we defined in Theorem 1.3, and note that $b_{-1}(s^1), d_{-1}(s^1)$ are the linear functions of $s^1$. For an arbitrary, but fixed $\hat{s}^1$, by the same way as we did to project $x_1$ in Section 1.2, we have:
\begin{align*}
  \text{Proj}_{x_{-2}} (F'(\hat{s}^1)) = \bigcup_{s^2 \in \{0,1,\ldots, m_2 - 1\}^{|P_2|}} F''(\hat{s}^1; s^2),
\end{align*}
where $F''(\hat{s}^1; s^2)$ have the same form as $F'(s^1)$, therefore, using Theorem 1.3 again, we have $F''(\hat{s}^1; s^2)$ can be written as:
\begin{align*}
  F'(\hat{s}^1; s^2) =
  \left\{ x_{-2} \in \mathbb{Z}^{n - 2}:~
  \begin{array}{lll}
  A_{-2} x_{-2} \leq b_{-2}(\hat{s}^1; s^2)& \\
  C_{-2} x_{-2} \equiv d_{-2}(\hat{s}^1; s^2)& \bmod ~ m_{-2} \\
  \end{array}
  \right\},
\end{align*}
where $A_{-2}, C_{-2}, m_{-2}, b_{-2}(\hat{s}^1; s^2), d_{-2}(\hat{s}^1; s^2)$ are defined the same as $A_{-1}, C_{-1}, m_{-1}, b_{-1}(s^1), d_{-1}(s^1)$ in Theorem 1.3.\\
\textbf{Note that} by the same analysis we did in Theorem 1.3, we have $A_{-2}, C_{-2}, m_{-2}$ are independent from $\hat{s}^1, s^2$, and by the way we adding slack variables $s^2$, we have $b_{-2}(\hat{s}^1; s^2), d_{-2}(\hat{s}^1; s^2)$ are linear functions for both $\hat{s}^1$ and $s^2$. \guanyi{I need to prove this step, but the notations seems too complex.} \\
Therefore, we have:
\begin{align*}
  \text{Proj}_{x_{-2}} (F) & =  \bigcup_{s^1 \in \{0,1,\ldots, m_1 - 1\}^{|P_1|}} \text{Proj}_{x_{-2}} (F'(s^1)), \\
  & = \bigcup_{s^1 \in \{0,1,\ldots, m_1 - 1\}^{|P_1|}} \bigcup_{s^2 \in \{0,1,\ldots, m_2 - 1\}^{|P_2|}} F''(s^1, s^2), \\
  & = \bigcup_{s^1 \in \{0,1,\ldots, m_1 - 1\}^{|P_1|}} \bigcup_{s^2 \in \{0,1,\ldots, m_2 - 1\}^{|P_2|}} 
  \left\{ x_{-2} \in \mathbb{Z}^{n - 2}:~
  \begin{array}{lll}
  A_{-2} x_{-2} \leq b_{-2}(s^1, s^2)& \\
  C_{-2} x_{-2} \equiv d_{-2}(s^1, s^2)& \bmod ~ m_{-2} \\
  \end{array}
  \right\},
\end{align*}
where $A_{-2}, C_{-2}, m_{-2}$ do not depend on $s^1, s^2$ and $b_{-2}(s^1,s^2), d_{-2}(s^1, s^2)$ are linear functions for $s^1, s^2$. \\
Therefore, repeat the steps above, then we have the projection of $F$ onto $x_{-k}$ is 
\begin{align*}
  & \text{Proj}_{x_{-k}} (F)\\
  = & \bigcup_{s^i \in \{0, 1, \ldots, m_i - 1\}^{|P_i|}}^{i \in \{1,\ldots, k\}}
  \left\{ x_{-k} : ~
  \begin{array}{ll}
  A_{-k} x_{-k} \leq b_{-k}(s^1, \ldots, s^k) & \\
  C_{-k} x_{-k} \equiv d_{-k}(s^1, \ldots, s^k)& \bmod \bar{m}_{-k}
  \end{array}
  \right\}
\end{align*}
where $A_{-k}, C_{-k}, \bar{m}_{-k}$ do not depend on $s^1, \ldots, s^k$ and $b_{-k}(s^1, \ldots, s^k),  d_{-k}(s^1, \ldots, s^k)$ are linear functions for $s^1, \ldots, s^k$.
\end{proof}

\subsection{Supplementary results}

%\begin{lemma} \label{lemma:cong-reduction-1}
%Consider the system of congruences in $\mathbb{Z}^n$
%\begin{eqnarray}
%c^j_1 u_1  +  c^j_{-1}x_{-1}  \equiv d^j \mod m^j, \, \, \forall j \in J. \label{eq:cong-reduction}
%\end{eqnarray}
%Let $m :=  \text{l.c.m}. (\{(m^j\}_{j \in J}).$  If $(\hat u_{1}, \hat x_{-1}) \in \mathbb{Z}^n$ is a solution to~\eqref{eq:cong-reduction}, then for any $s\in \mathbb{Z},$  $(\hat u_{1} + s m, \hat x_{-1})$ is a solution to~\eqref{eq:cong-reduction}.
%\end{lemma}
%
%\begin{proof}
%Since $(\hat u_{1}, \hat x_{-1})$ is a solution to~\eqref{eq:cong-reduction}
%\begin{eqnarray}
%c^j_1 \hat u_1  +  c^j_{-1} \hat x_{-1} -  d^j  \equiv 0 \mod m^j, \, \, \forall j \in J.  \label{eq:cong-reduction-1}
%\end{eqnarray}
%The  definition of $m$ and the fact that $c^j_1, s \in  \mathbb{Z}$ gives
%\begin{eqnarray}
%c^j_1 s m   \equiv 0 \mod m^j, \, \, \forall j \in J.   \label{eq:cong-reduction-2}
%\end{eqnarray}
%Combining~\eqref{eq:cong-reduction-1} and\eqref{eq:cong-reduction-2} gives
%\begin{eqnarray}
%c^j_1 \hat u_1  +  c^j_{-1} \hat x_{-1} -  d^j  +  c^j_1 s m  \equiv 0 \mod m^j, \, \, \forall j \in J.  \label{eq:cong-reduction-3}
%\end{eqnarray}
%Combining the terms  $c^j_1 \hat u_1 $ and $c^j_1 s m$  in~\eqref{eq:cong-reduction-3}  gives
%\begin{eqnarray*}
%c^j_1 (\hat u_1  + s m) +  c^j_{-1} \hat x_{-1} -  d^j     \equiv 0 \mod m^j, \, \, \forall j \in J.
%\end{eqnarray*}
%and the proof is complete.
%\end{proof}

Recall the notation $\bmod(z,  m)$ to mean $z$ is reduced modulo $m$ to a unique integer in $\{0, 1, \ldots,  m - 1 \}.$

\begin{lemma} \label{lemma:cong-reduction-2}
Consider the system of congruences in $\mathbb{Z}^n$
\begin{eqnarray}
c^j_1 u_1  +  c^j_{-1}x_{-1}  \equiv d^j \mod{m^{j}}, \, \, \forall j \in J. \label{eq:cong-reduction}
\end{eqnarray}
Let $m :=  \text{l.c.m}. (\{(m^j\}_{j \in J}).$   Then $(\hat u_{1}, \hat x_{-1}) \in \mathbb{Z}^n$ is a solution to~\eqref{eq:cong-reduction} if and only if $(\bmod(\hat u_{1}, m), \hat x_{-1})$ is a solution to~\eqref{eq:cong-reduction}.
\end{lemma}

\begin{proof} Let $r := \bmod( \hat u_1, m)$; then there exists $s\in \Z$ such that $\hat u_{1} + s m = r$ with $r \in \{0, 1, \ldots, m - 1  \}$. Observe that

$$
\begin{array}{rl}
& c^j_1 \hat u_1  +  c^j_{-1} \hat x_{-1} -  d^j  \equiv 0 \mod m^j, \, \, \forall j \in J \\
\Leftrightarrow & c^j_1 (\hat u_1 +sm) +  c^j_{-1} \hat x_{-1} -  d^j  \equiv 0 \mod m^j, \, \, \forall j \in J \\
\Leftrightarrow  & c^j_1 r  +  c^j_{-1} \hat x_{-1} -  d^j  \equiv 0 \mod m^j, \, \, \forall j \in J.
\end{array}
$$
where first equivalence follows from the fact that $c^j_1sm \equiv 0 \mod m$ and hence $c^j_1sm \equiv 0 \mod m^j$. The second equivalence follows from the definition of $r$.
%
%  The result is now immediate by using $r$ for $\hat u_{1} + s m$ in Lemma~\ref{lemma:cong-reduction-1}.
\end{proof}

\subsection{Numerical Example}
Consider an integer programming problem $F$ as:
\begin{align*}
\begin{array}{llllll}
  \min        & z &      & & \\
  \text{s.t.} & z &      & - x_2 & \geq 0 \\
              &   & 2x_1 & + x_2 & \geq 13 \\
              &   & -5x_1& - 2x_2& \geq -30 \\
              &   & -x_1 & + x_2 & \geq 5 \\
\end{array}
\end{align*}
Then let all the coefficients of $x_1$ be the same, we have $q_1 = \text{l.c.m}(2, 5, 1) = 10$ and transfer the original integer programming problem into
\begin{align*}
\begin{array}{llllll}
  \min        & z &      & & \\
  \text{s.t.} & z &      & - x_2 & \geq 0 \\
              &   & 10x_1 & + 5x_2 & \geq 65 \\
              &   & -10x_1& - 4x_2 & \geq -60 \\
              &   & -10x_1& + 10x_2& \geq 50 \\
\end{array}
\end{align*}
And transform the problem above into the standard form as:
\begin{align*}
\begin{array}{llllll}
  \min        & z &       & & \\
  \text{s.t.} & z &       & - x_2 & \geq 0  & \\
              &   & 10x_1 &       & \geq 65 &- 5x_2 \\
              &   & -10x_1&       & \geq -60&+ 4x_2  \\
              &   & -10x_1&       & \geq 50 &- 10x_2 \\
\end{array}
\end{align*}
We have $Z: z - x_2 \geq 0$, $P: 10x_1 \geq 65 - 5x_2$ and $N: -10x_1 \geq -60+ 4x_2, ~ -10x_1 \geq 50 - 10x_2$, therefore $P \neq \emptyset, N \neq \emptyset$ and we are in Case 1. Then combine each inequality constraints in set $P$ and set $N$ as:
\begin{align*}
\begin{array}{llllllll}
  \min        & z &       & & \\
  \text{s.t.} & z &       & - x_2 & \geq 0     & \\
              & 60& -4x_2 &       & \geq 10x_1 & \geq & 65 & - 5x_2 \\
              &-50&+10x_2 &       & \geq 10x_1 & \geq & 65 & - 5x_2 \\
\end{array}
\end{align*}
Then add slack variable $s^1 \in \mathbb{Z}_+$ to the inequality constraints in set $P$ such that $10 x_1  = 65 - 5x_2 + s^1$. Since $m_1 = \text{l.c.m}\{10\} = 10$. Therefore, we have the projection of $F$ onto $x_{-1} = x_2$ as:
\begin{align*}
  \text{Proj}_{x_{-1}}(F) & = \bigcup_{s^1 \in \{ 0,1,\ldots, 9 \}}
  \left\{ z \in \mathbb{Z}:~ 
  \begin{array}{llllllll}
   z &       & - x_2 & \geq 0     \\
   60& -4x_2 &       & \geq 65  - 5x_2 + s^1 \\
   -50&+10x_2&       & \geq 65  - 5x_2 + s^1 \\
   65 &      & -5x_2 + s^1 & \equiv 0 ~ \bmod ~ 10 \\
  \end{array}
  \right\} \\
  & = \bigcup_{s^1 \in \{ 0,1,\ldots, 9 \}}
  \left\{ z \in \mathbb{Z}:~ 
  \begin{array}{llll}
  z & - x_2 & \geq & 0 \\
    &   x_2 & \geq & 5 + s^1 \\
    & 15x_2 & \geq & 115 + s^1 \\
    & 5 x_2 & \equiv & 5 + s^1 ~ \mod ~ 10 \\
  \end{array}
  \right\}.
\end{align*}
Then we have project out the first variable $x_1$, then for $x_2$, first find the least common multiplier $q_2 = \text{l.c.m}(1, 15, -(-1), 5) = 15$, therefore $\text{Proj}_{x_{2}} (F)$ is:
\begin{align*}
  \text{Proj}_{x_{-1}} (F) = \bigcup_{s^1 \in \{ 0,1,\ldots, 9 \}}
  \left\{ z \in \mathbb{Z}:~
  \begin{array}{llll}
  15z & - 15x_2 & \geq & 0 \\
      & 15x_2 & \geq & 75 + 15s^1 \\
      & 15x_2 & \geq & 115 + s^1 \\
      & 15x_2 & \equiv & 15 + 3s^1 ~ \mod ~ 30 \\
  \end{array}
  \right\}.
\end{align*}
We have $Z_2 :\emptyset, ~ P_2: 15x_2 \geq 75 + 15s^1, 15x_2 \geq 115 + s^1$ and $N_2: 15 z - 15 x_2$, therefore $P_2 \neq \emptyset, N_2 \neq \emptyset$ and we are in Case 1. Then combine each inequality constraints in set $P_2$ and set $N_2$ as:
\begin{align*}
  \text{Proj}_{x_{-1}} (F) & = \bigcup_{s^1 \in \{ 0,1,\ldots, 9 \}}
  \left\{ z \in \mathbb{Z}:~
  \begin{array}{llllll}
  15z &       & \geq   & 15 x_2 & \geq 75 + 15 s^1 \\
  15z &       & \geq   & 15 x_2 & \geq 115 + s^1 \\
      & 15x_2 & \equiv & 15 + 3s^1 & \mod ~ 30 \\
  \end{array}
  \right\}.
\end{align*}
Then add slack variable $s^2_1, s^2_2$ to the inequality constraints in set $P_2$, such that:
\begin{align*}
  15 x_2 & = 75 + 15 s^1 + s^2_1, \\
  15 x_2 & = 115 + s^1 + s^2_2.
\end{align*}
Since $m_2 = l.c.m(15, 30) = 30$. Therefore, we have the projection of $F$ onto $x_{-2}$ as:
\begin{align*}
  \text{Proj}_{x_{-2}} (F) & = \bigcup_{\substack{s^1 \in \{0,\ldots, 9\} \\ s^2 \in \{0, \ldots, 29\}^2}} 
  \left\{ z \in \mathbb{Z}: ~ 
  \begin{array}{llllll}
  15 z & \geq & 75 + 15 s^1 + s^2_1 & \\
  15 z & \geq & 115 + s^1 + s^2_2 & \\
  0 & \equiv  & -60 - 12s^1 - s^2_1 & \bmod ~ 30 \\
  0 & \equiv  & -100 + 2s^1 - s^2_2 & \bmod ~ 30 \\
  0 & \equiv  & 75 + 15 s^1 + s^2_1 & \bmod ~ 15 \\
  0 & \equiv  & 115 + s^1 + s^2_1   & \bmod ~ 15 \\
  \end{array}
  \right\}.
\end{align*}
